# Supplementary material for: Controllable Complementarity: Subjective Preferences in Human-AI Collaboration
Source: arXiv:2503.05455 source file (2025-03-07)
Supplement: Supplementary file 1 [file appendix.tex]

\appendix

\section{Overcooked} \label{sec:overcooked_environment}

\newcommand{\figheight}{2.3cm} % Define a macro for the consistent figure height

The five Overcooked layouts, as originally proposed by \cite{carroll2019utility}, are shown in Figure~\ref{fig:overcooked_layouts}. The environment layouts remain unchanged in our implementation; however, we extended the episode length to be 1,000 steps. Both agents receive a baseline reward of 1.0 when a dish is delivered.

\begin{figure}
    \centering
    % Top row: 5 images
    \begin{subfigure}{0.5\linewidth}
        \centering
        \includegraphics[height=1.88cm]{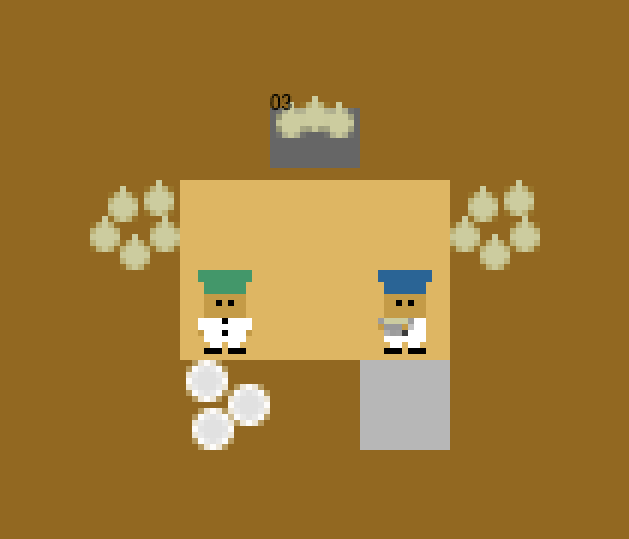}
        \caption{Cramped Room}
    \end{subfigure}%
    % \hspace{0.5cm}
    \begin{subfigure}{0.5\linewidth}
        \centering
        \includegraphics[height=\figheight]{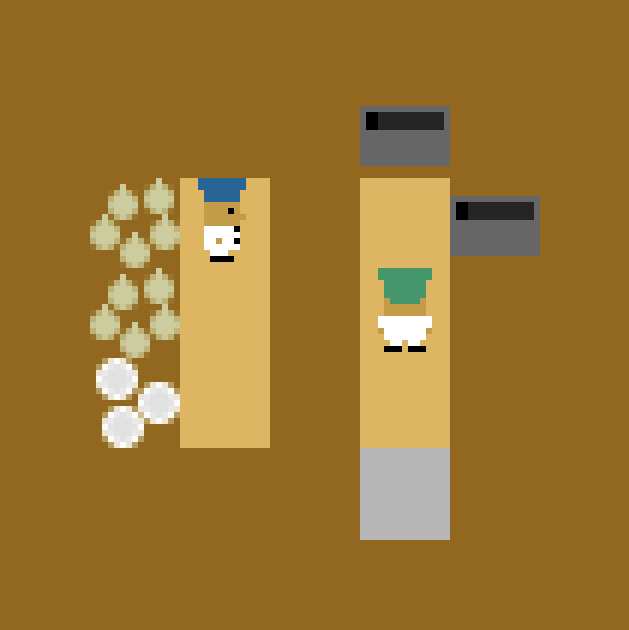}
        \caption{Forced Coordination}
    \end{subfigure}% 
        \vspace{1em}
    % \hspace{0.1cm}
    \begin{subfigure}{0.5\linewidth}
        \centering
        \includegraphics[height=\figheight]{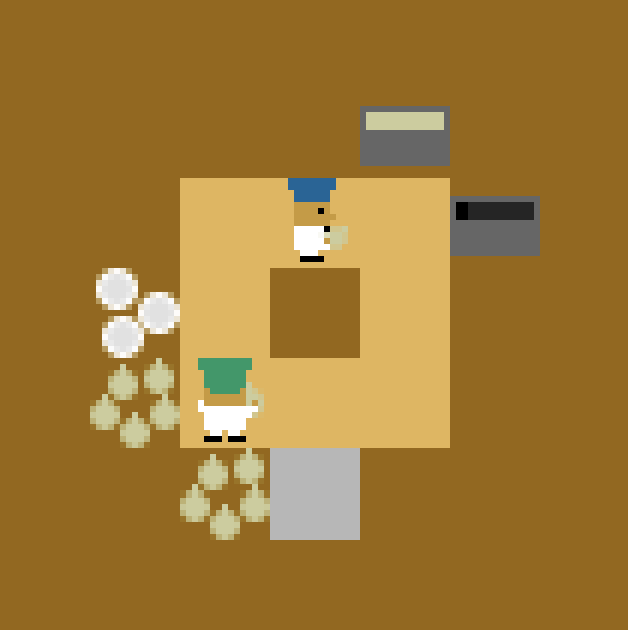}
        \caption{Coordination Ring}
    \end{subfigure}%
    % \vspace{1em}
    % \hspace{0.1cm}
    \begin{subfigure}{0.5\linewidth}
        \centering
        \includegraphics[height=\figheight]{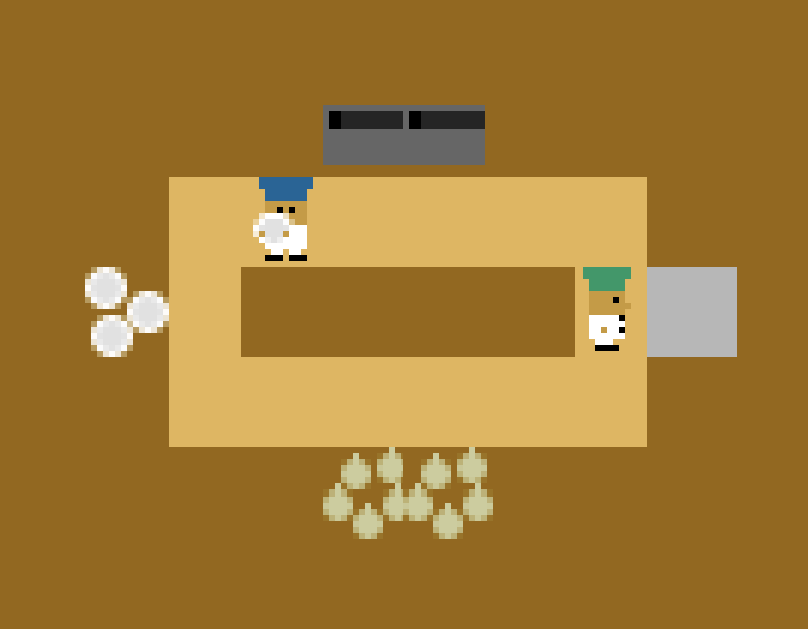}
        \caption{Counter Circuit}
    \end{subfigure}%
        \vspace{1em}

    % \hspace{0.1cm}
    \begin{subfigure}{0.5\linewidth}
        \centering
        \includegraphics[height=\figheight]{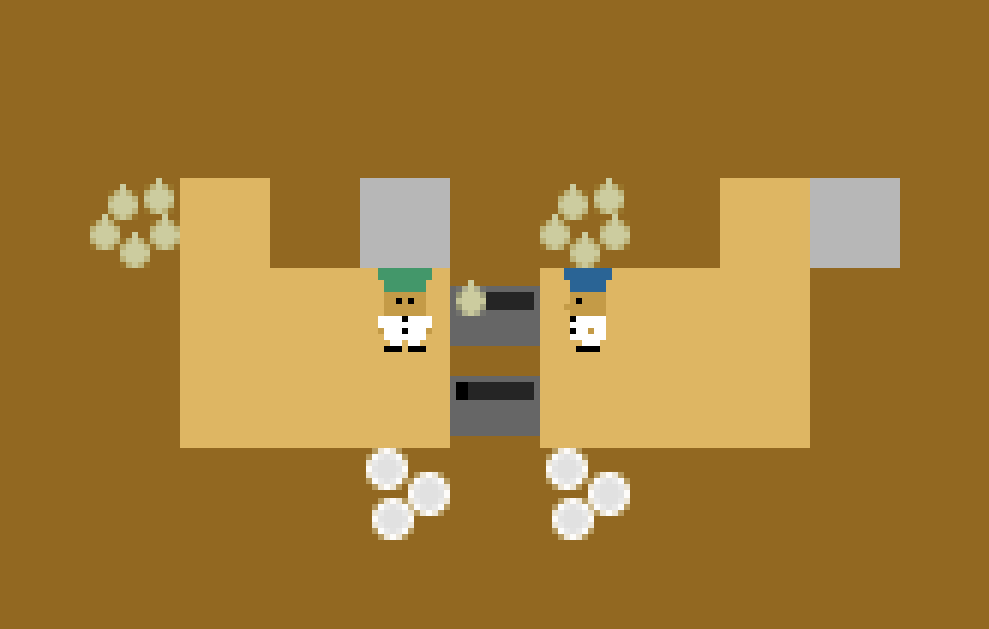}
        \caption{Asymmetric Advantages}
    \end{subfigure}

    \caption{The five overcooked layouts. In our experiments, the AI always takes the role of the chef in the green hat.}
    
    \label{fig:overcooked_layouts}

\end{figure}

\subsection{Training}

All policies are trained in a self-play paradigm with the Proximal Policy Optimization (PPO) algorithm \cite{schulman_proximal_2017}. We use a recurrent architecture, where the encoded observation of the environment (a concatenation of feature vectors) is first passed through an LSTM \cite{hochreiter1997long} with a cell size of 256 units. The body of the network consists of a three-layer multilayer perceptron (MLP), each layer with input and output size of 256. Each layer is separated by a ReLU activation. Finally, we have a single-layer MLP for each the policy and critic networks, which output the action distribution and value function, respectively. 

We trained a separate agent for each of the five Overcooked layouts. The key parameters are a discount rate of $\gamma=0.99$, a learning rate of $0.0008$, GAE-$\lambda$ of 0.99, value function loss coefficient of 0.5, and entropy coefficient of 0.01. We use 15 parallel workers for data collection and five concurrent environments per worker. These parameters were selected by conducting a grid search for the standard self-play policy and we use the same parameters on each layout. The same parameters were kept for training the BS policies. After training for 500 million policy steps (250 million environment steps), we select the best checkpoint for each trial.

\section{Manipulating BS Agent Behavior} \label{sec:BS_behavior}

We illustrate the effect of manipulating the $\omega$ weights in an BS policy in simulation. Beyond observing objective performance, it is critical that BS policies respond appropriately when we try to alter their behavior at inference time. Figure~\ref{fig:weight_manipulations} illustrates the wide variation in behavior we observe in simulation. In simulation and across layouts, we manipulate the $\omega$ weights for one of two policies and leave the other set to $\omega=0$. We then measure the overall performance as well as the amount of behavior-related tasks the policy accomplishes: for $\omega_1$ and $\omega_3$ we measure the number of dishes that agent delivers and for $\omega_2$ we count the number of onions that agent puts in the pot. 

\begin{figure*}
%     \centering
%     \begin{subfigure}{\linewidth}
%         \centering
%         \includegraphics[width=0.58\textwidth]{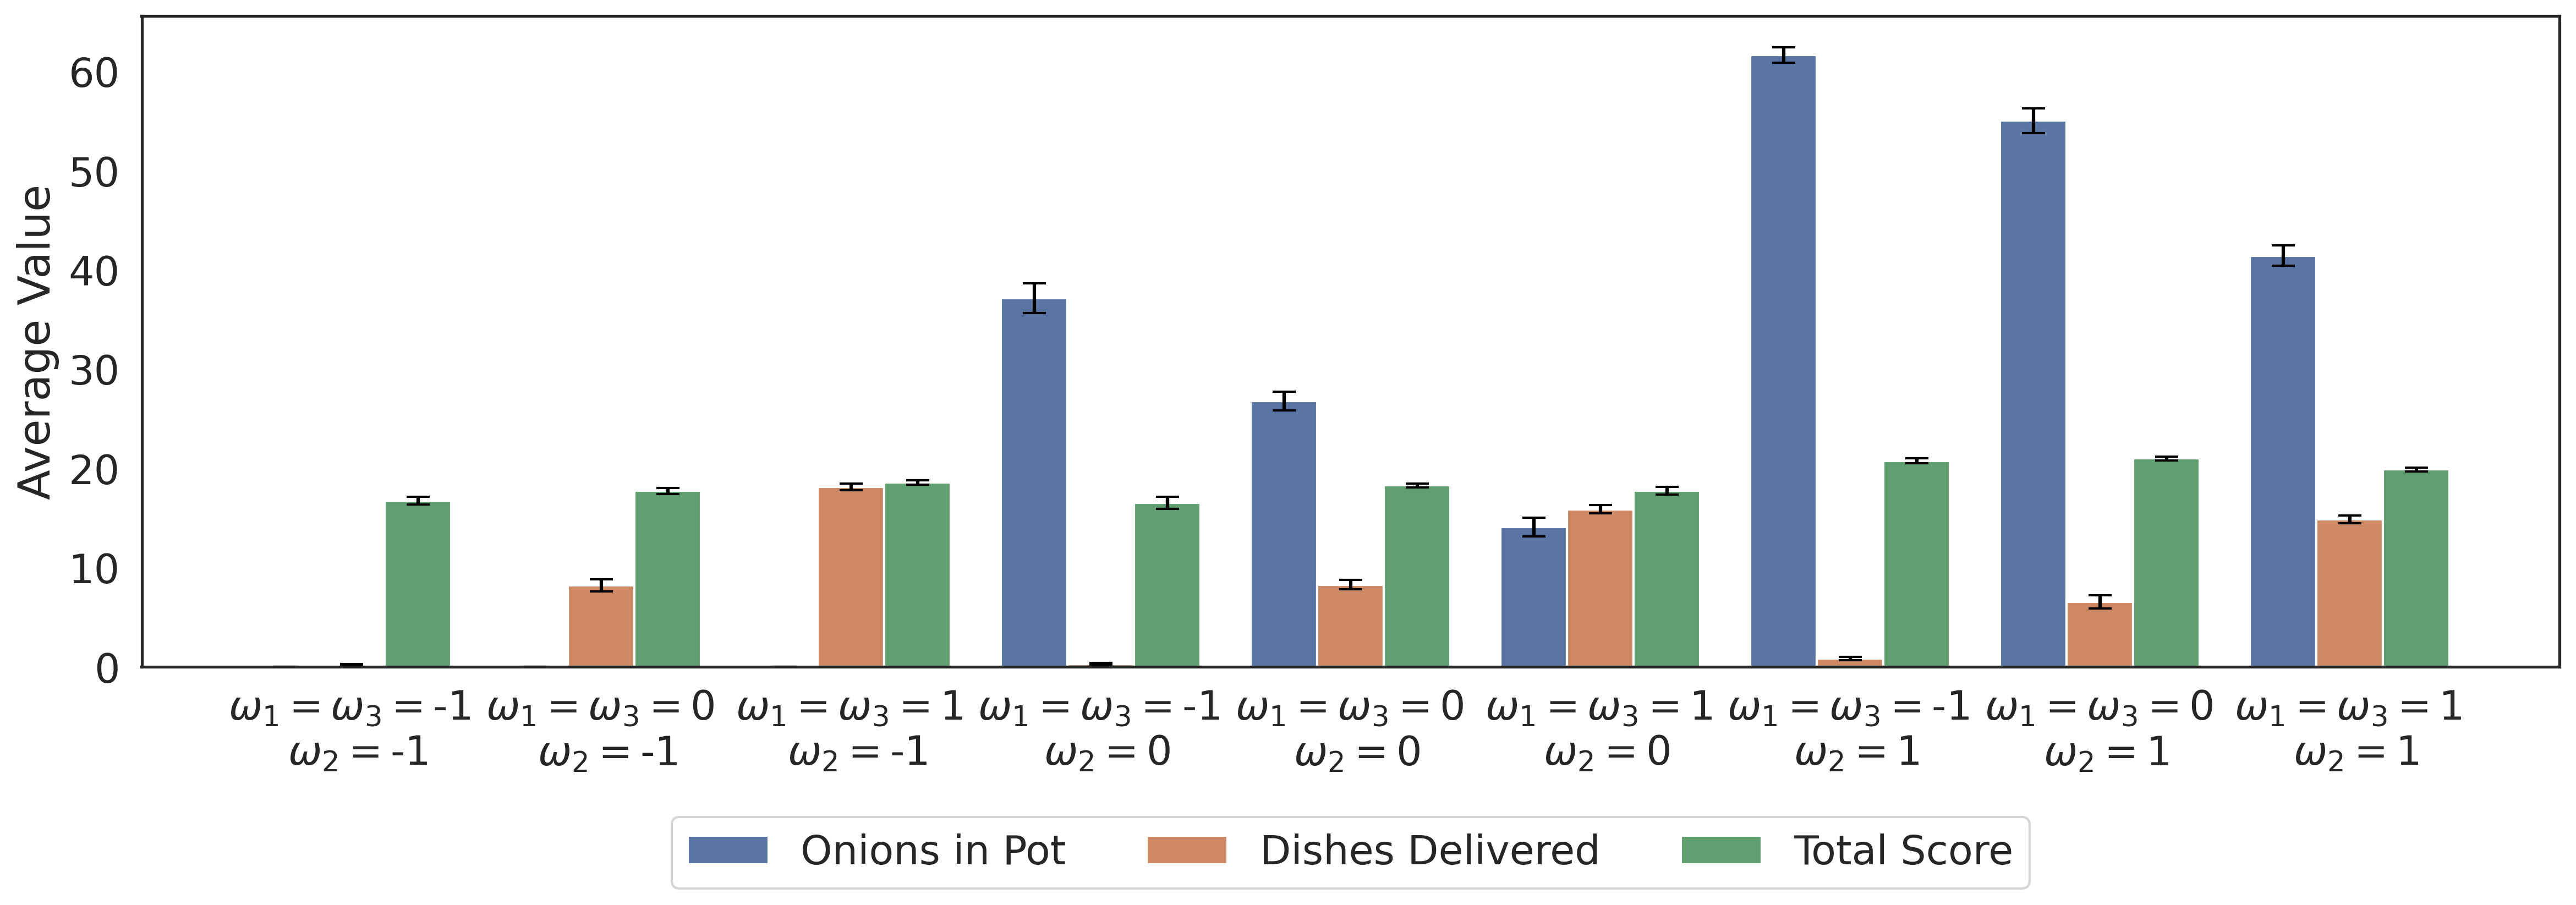}
%         \caption{Cramped Room}
%     \end{subfigure} \\
%         % \vspace{1em}

%     % \hspace{0.1cm}
%     \begin{subfigure}{\linewidth}
%         \centering
%         \includegraphics[width=0.58\textwidth]{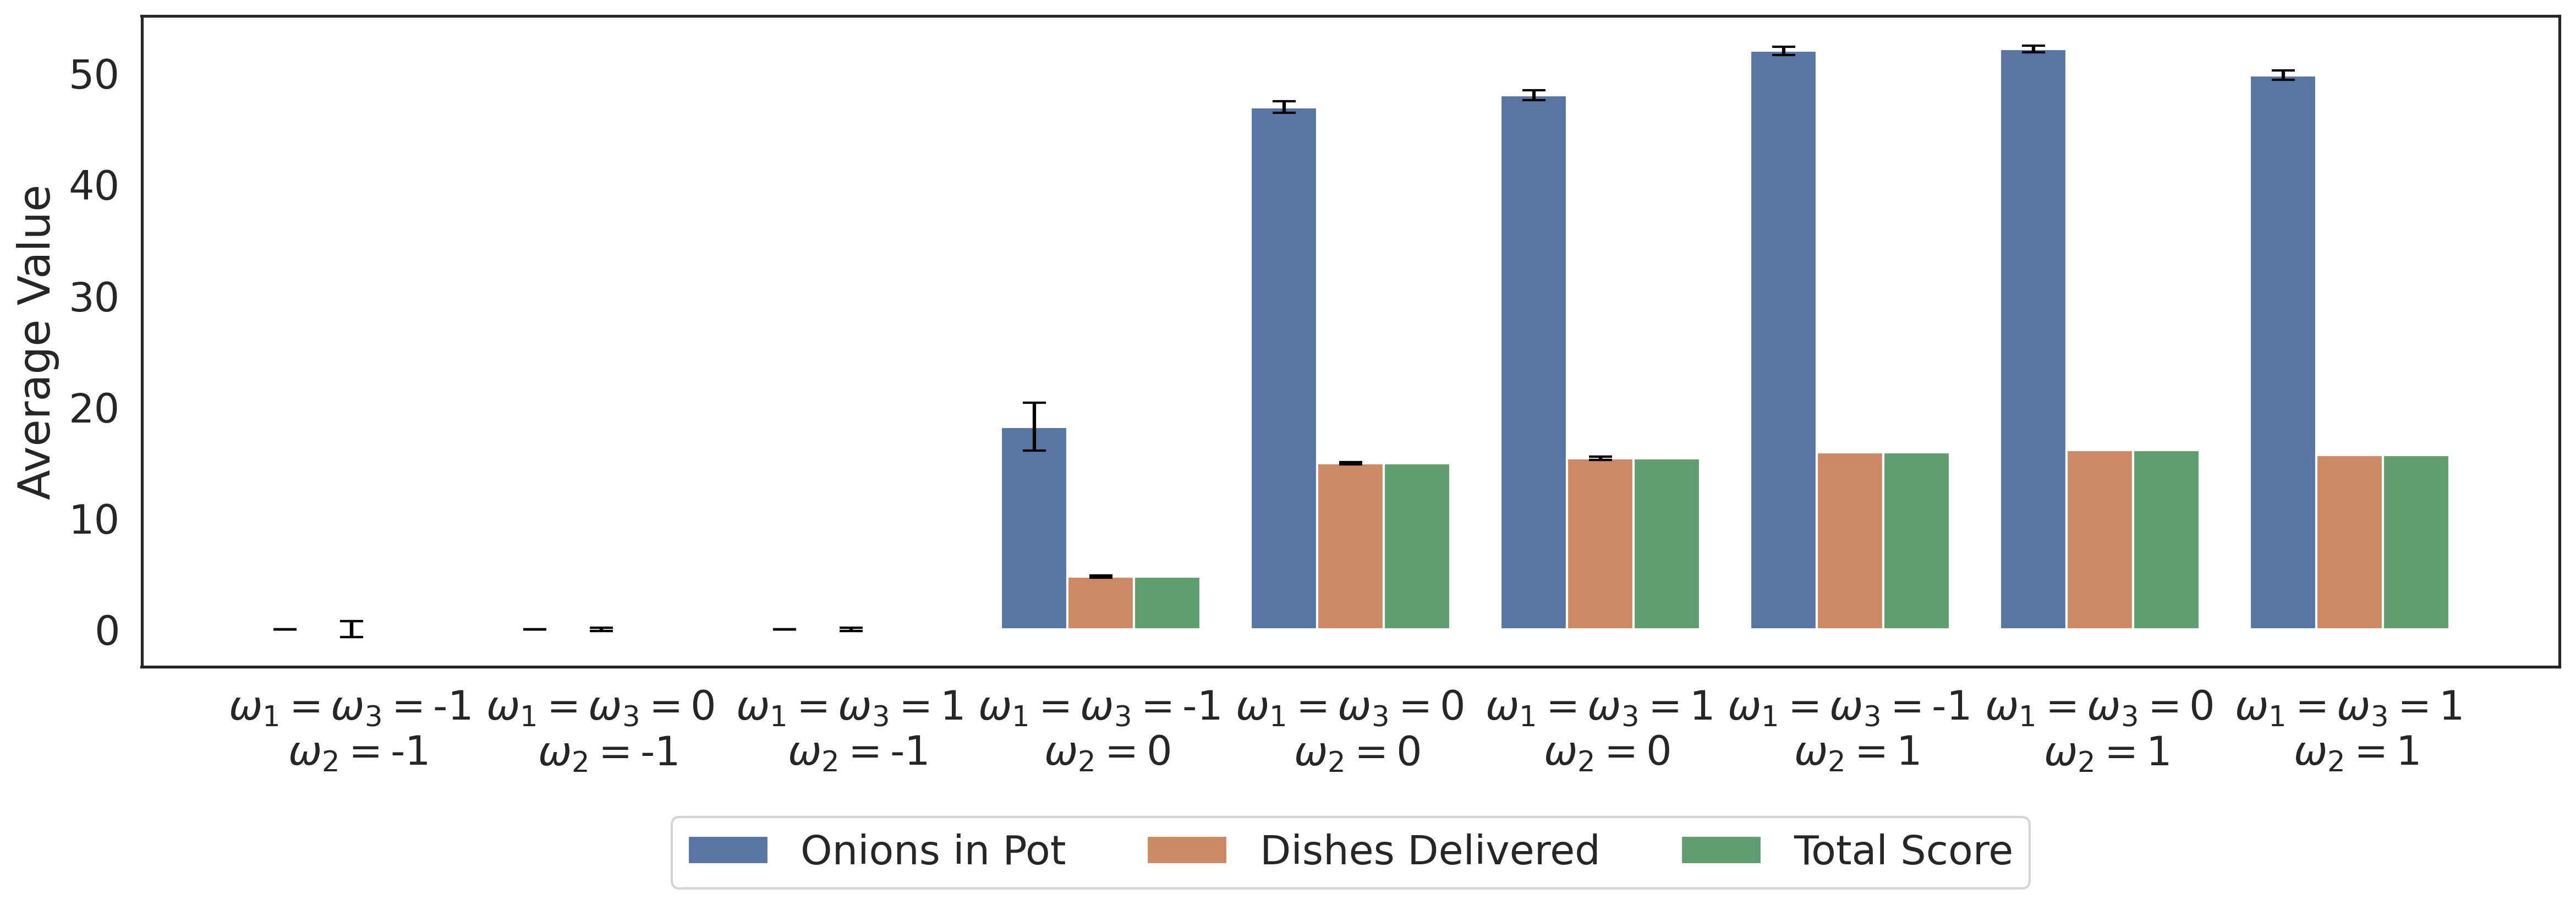}
%         \caption{Forced Coordination}
%     \end{subfigure} \\
%         % \vspace{1em}
%     % \hspace{0.1cm}
%     \begin{subfigure}{\linewidth}
%         \centering
%         \includegraphics[width=0.58\textwidth]{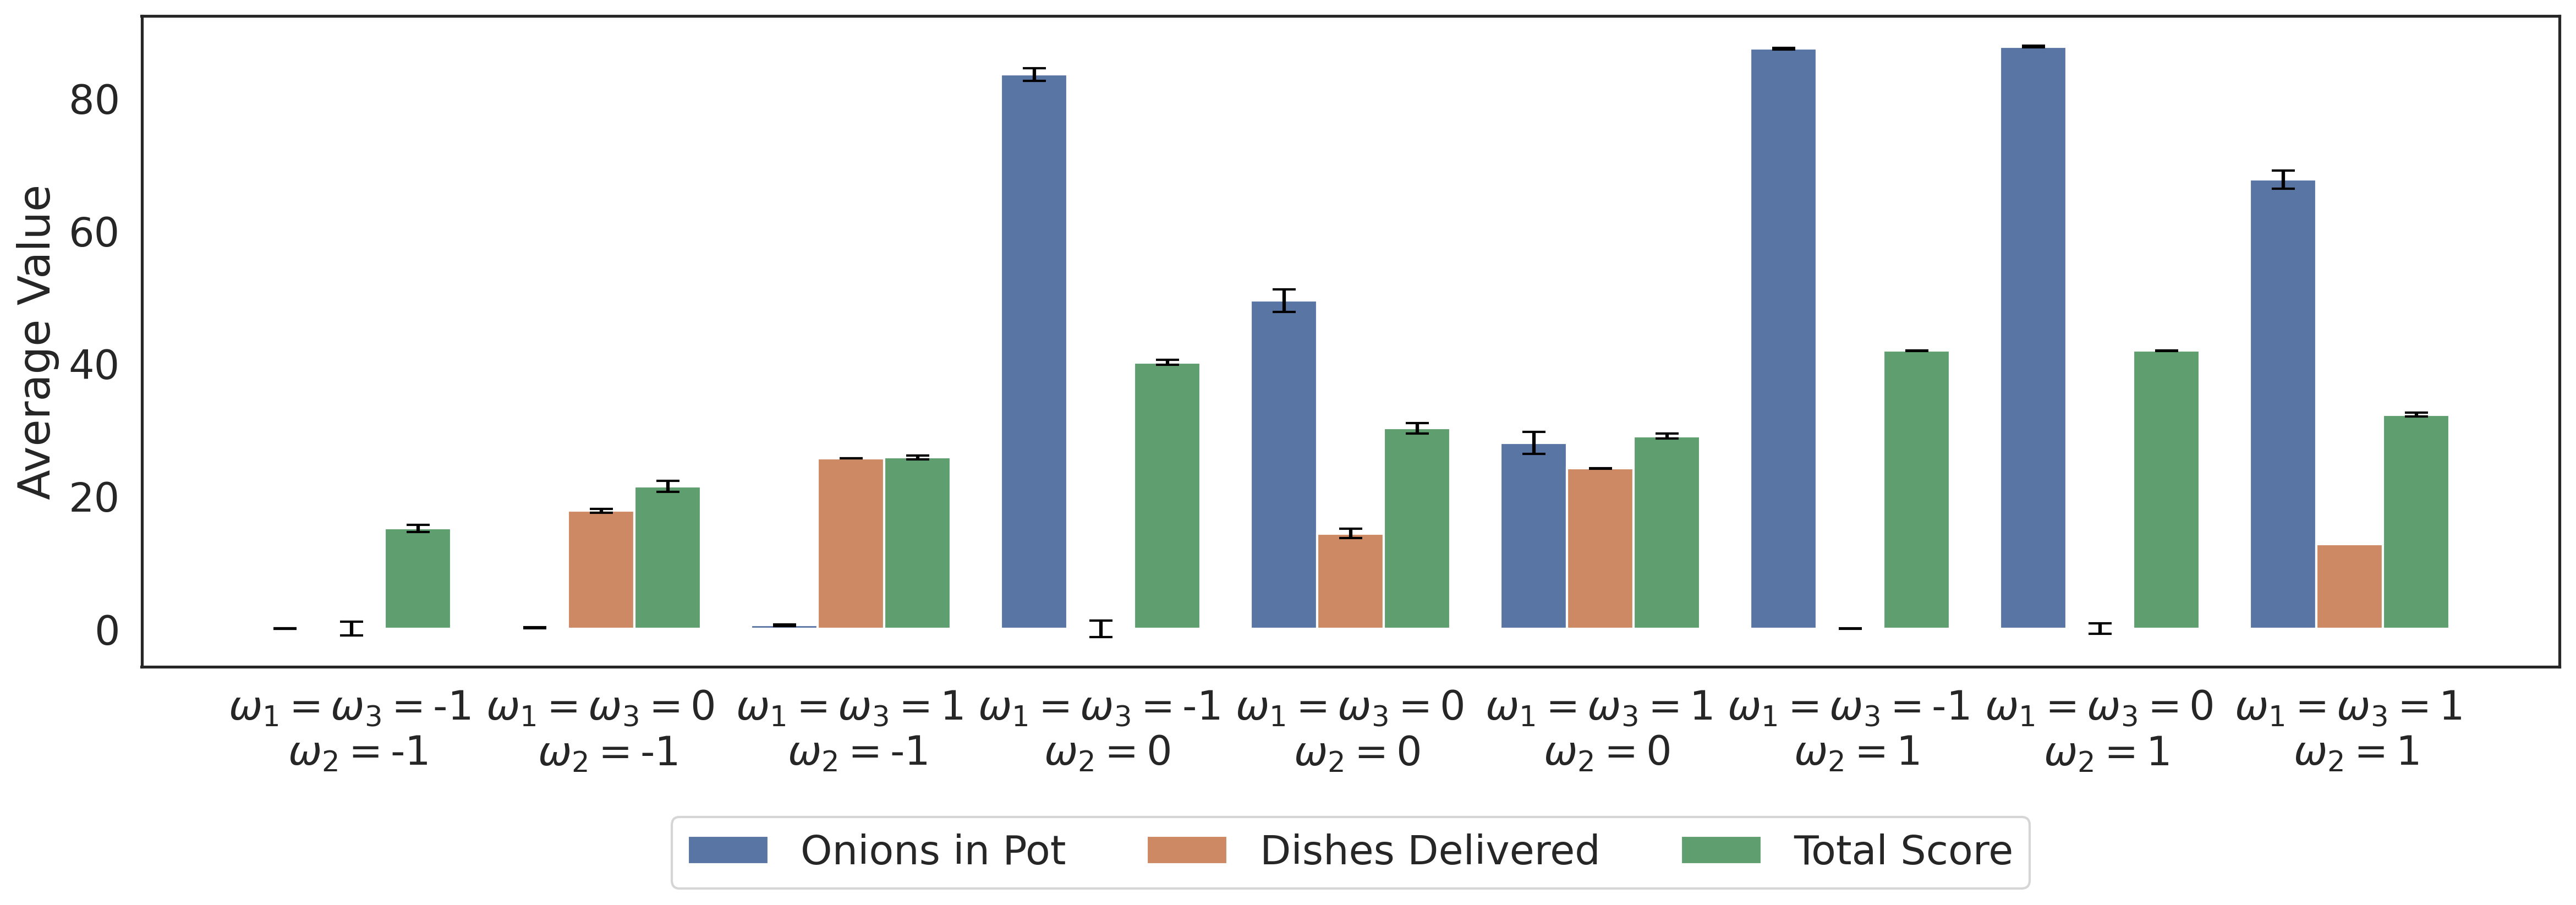}
%         \caption{Coordination Ring}
%     \end{subfigure}\\
%     % \hspace{0.1cm}
%     \begin{subfigure}{\linewidth}
%         \centering
%         \includegraphics[width=0.58\textwidth]{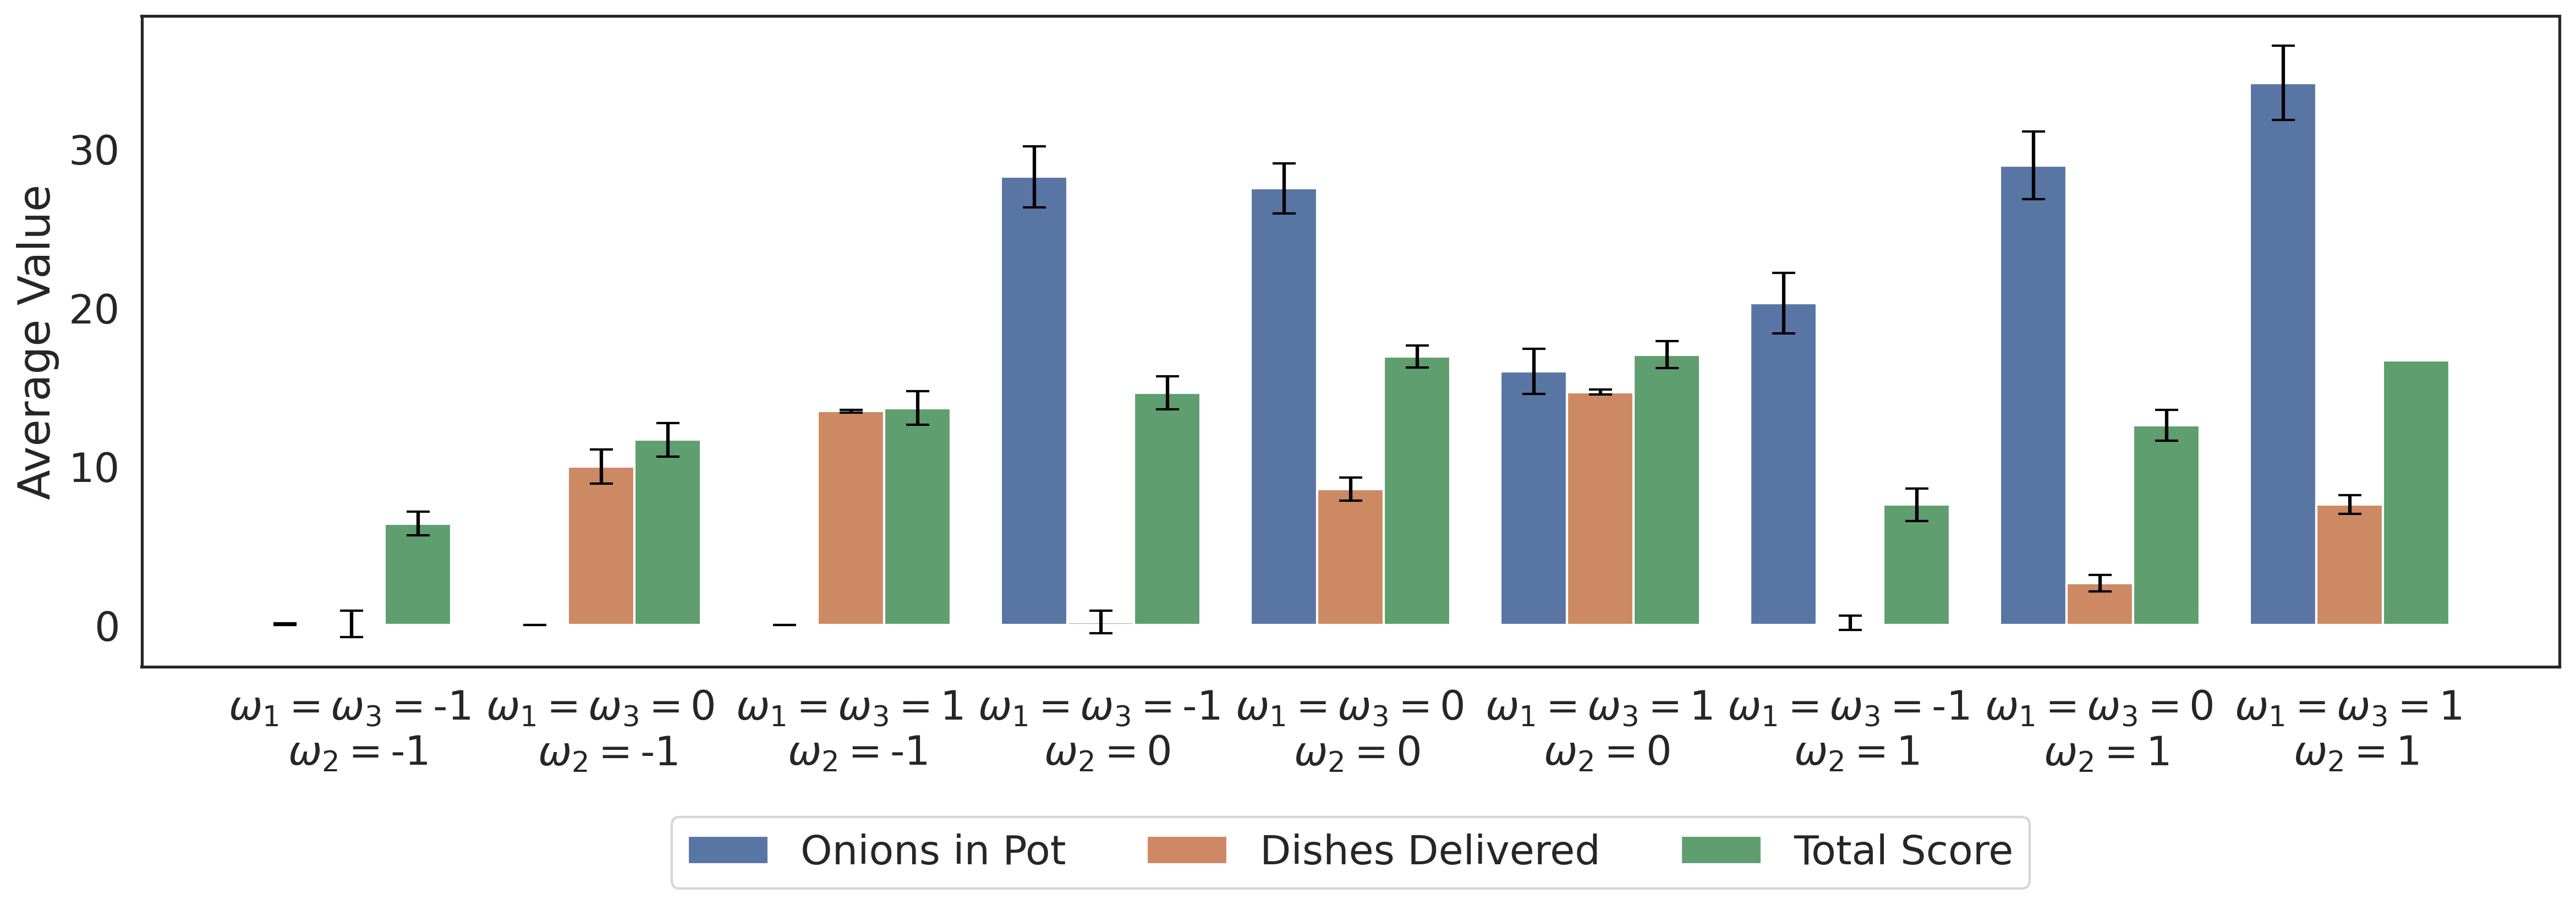}
%         \caption{Counter Circuit}
%     \end{subfigure}\\

%     % \hspace{0.1cm}
%     \begin{subfigure}{\linewidth}
%         \centering
%         \includegraphics[width=0.58\textwidth]{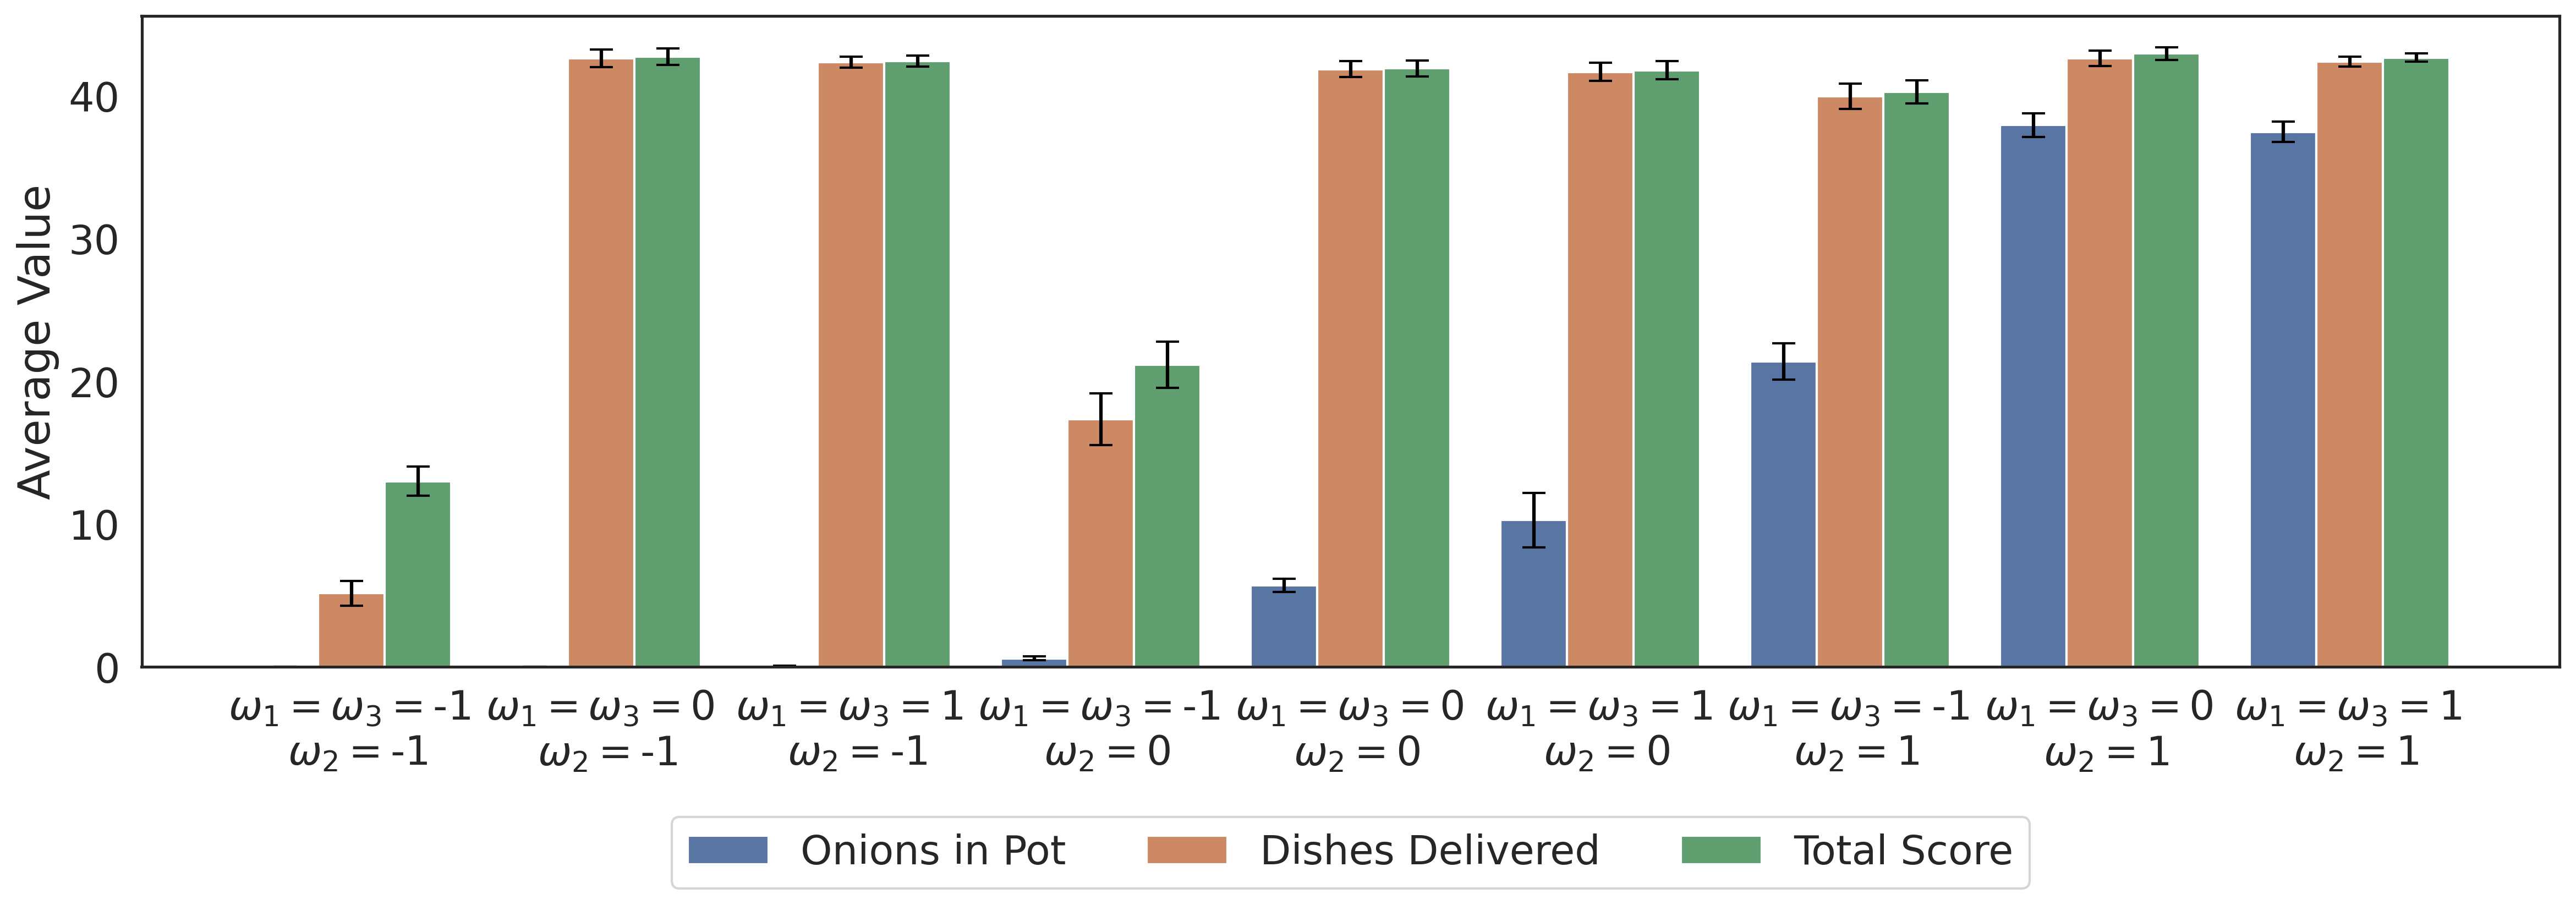}
%         \caption{Asymmetric Advantages}
%     \end{subfigure}

    \includegraphics[width=\textwidth]{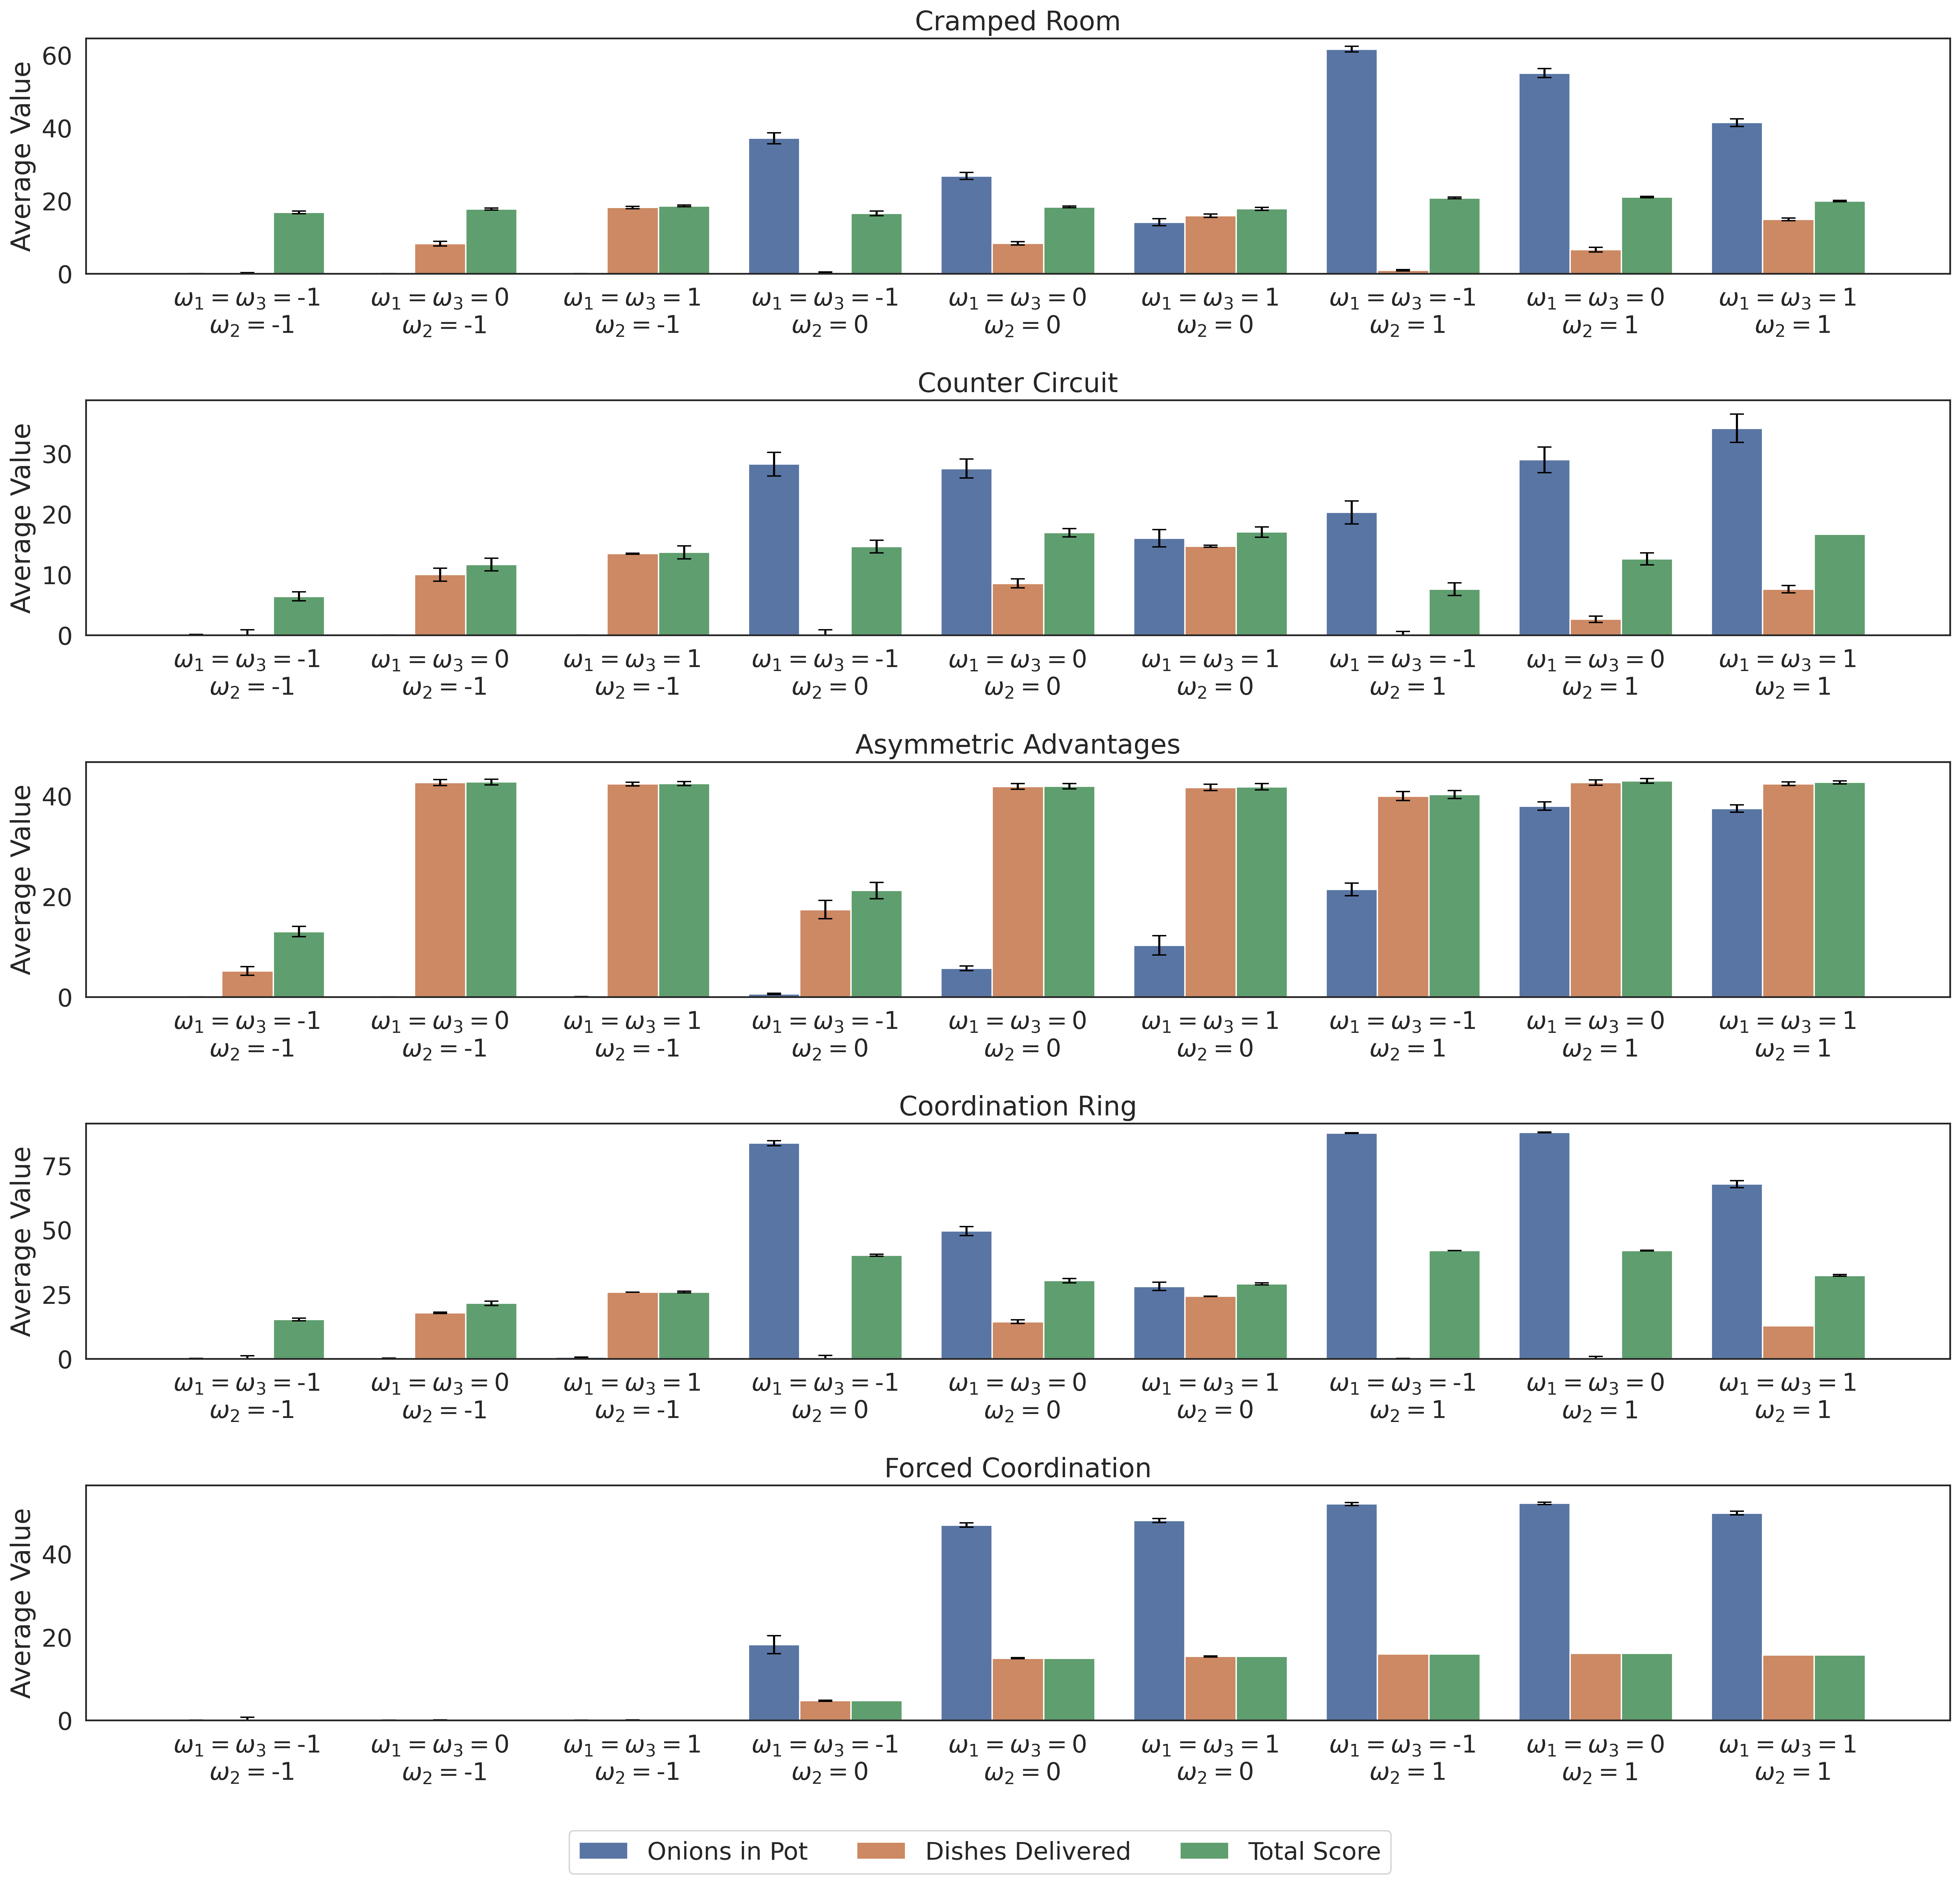}

    \caption{Across layouts, we set $\omega=0$ for one agent and manipulate the values for the other agent and track its behavior. As in the human control experiment in Section~5, we tie the values of $\omega_1$ and $\omega_3$ together (corresponding to plating and delivering dishes), while $\omega_2$ (putting onions in the pot) varies independently. We select values from $\{-1, 0, 1\}$ for each and collect data over 25 episodes per weight setting.} 
    
    \label{fig:weight_manipulations}

\end{figure*}

We see significant variation across all layouts in the behavior exhibited with different wights. Indeed, with $\omega_2=-1$, the agent completely stops placing onions in the pot. In the vast majority of instances, we see dish delivery decrease with $\omega_1$ and $\omega_3$ reductions. There are some notable caveats and exceptions. The clearest is in the poor performance and controllability in the Forced Coordination environment. In this setting, the only possible way to achieve any reward is for the agent to do every task (recall it is always on the right hand side with the pots and delivery area). As such, there are minimal variations between when the agent has deemed it valuable enough to successfully complete the task.

% \section{Experiment 1 Design}

% \section{Experiment 2 Design}
